# Supplementary material for: Probing Permanent Dipoles in CdSe Nanoplatelets with Transient Electric Birefringence
Source: arXiv:1912.02679 source file (2019-12-05)
Supplement: Supplementary file 1 [file supp_info.pdf]

# Supplementary information for: Probing Permanent Dipoles in CdSe Nanoplatelets with Transient Electric Birefringence

Ivan Dozov,[1,*] Claire Goldmann,[1] Patrick Davidson,[1] and Benjamin Abécassis[1,2,†]

[1] *Laboratoire de Physique des Solides, Université Paris-Saclay, CNRS, Université Paris-Sud, UMR 8502, 91405 Orsay, France.*

[2] *Univ Lyon, ENS de Lyon, CNRS UMR 5182, Université Claude Bernard Lyon 1, Laboratoire de Chimie, F69342, Lyon, France*

(Dated: November 28, 2019)

## I. GENERAL FORMULA FOR THE FIELD-INDUCED ORIENTATIONAL ORDER PARAMETER:

When the dispersion is isotropic in the absence of field and the particles have cylindrical symmetry around some particle axis $\mathbf{p}$, the induced order $S(E)$ is given by:

$$S(E) = \frac{3}{2}\langle\cos^2\Theta\rangle - \frac{1}{2} = \frac{1}{2}\frac{\int_{-1}^{1}\left(3\cos^2\Theta - 1\right)\exp\left(-U^P(\cos\Theta)/(kT)\right)d\cos\Theta}{\int_{-1}^{1}\exp\left(-U^P(\cos\Theta)/(kT)\right)d\cos\Theta}, \tag{1}$$

where $\Theta$ is the angle between $\boldsymbol{e}$ and $\boldsymbol{p}$, $k$ is the Boltzmann constant, $T$ is the temperature, and the brackets denote a statistical average.

## II. RISE BEHAVIOR OF THE BIREFRINGENCE UNDER FIELD PULSES:

In general, three distinct relaxation times are involved in the rotational relaxation process under field. The first one, $1/(6D^r_\perp)$, is the time related to the reorientation of a second rank tensor, namely the polarizability $\alpha$ of the particle, under a DC field. The two additional terms, $1/(2D^r_\perp)$ and $1/(D^r_\perp + D^r_\parallel)$ are respectively the relaxation times of the longitudinal and transverse components of the permanent dipole moment of the particle [1]:

$$\begin{aligned}\frac{\Delta n^{\rm on}(t)}{\Delta n^e(E)} = 1 - \frac{3p_\parallel}{2(p_\parallel - p_\perp + q)}\exp\left(-2D^r_\perp t\right) \\ + \frac{6D^r_\perp p_\perp}{(5D^r_\perp - D^r_\parallel)(p_\parallel - p_\perp + q)}\exp\left(-(D^r_\perp + D^r_\parallel)t\right) \\ + \left(p_\parallel/2 + p_\perp - q - \frac{6D^r_\perp p_\perp}{5D^r_\perp - D^r_\parallel}\right)\frac{1}{(p_\parallel - p_\perp + q)}\exp\left(-6D^r_\perp t\right)\end{aligned} \tag{2}$$

A simpler treatment of the data is possible when $D^r_\parallel \simeq D^r_\perp$ or when $D^r_\parallel \gg D^r_\perp$. In both cases, only two exponentials are needed to fit the rise curve:

$$\Delta n^{on}(t) = \Delta n^e(E)\left[1 - \frac{3\beta}{2(\beta+1)}\exp(-2D^r_\perp t) + \frac{\beta-2}{2(\beta+1)}\exp(-6D^r_\perp t)\right], \tag{3}$$

where $\beta$ is respectively $(p_\parallel - p_\perp)/q$ and $p_\parallel/(q - p_\perp)$ in each case.
However, the numerical estimate of the diffusion coefficients yields $D^r_\parallel \simeq 3D^r_\perp$ for our CdSe particles so that neither approximations apply. In our case, a simpler approach consists in comparing the two areas limited by the on- and off- curves i.e. the integrals:

$$I^{\rm on} = \int_0^\infty \left(\Delta n^e(E) - \Delta n^{\rm on}(t)\right)dt; \quad I^{\rm off} = \int_0^\infty \Delta n^{\rm off}(t)dt \tag{4}$$

*Electronic address: ivan.dozov@u-psud.fr
†Electronic address: benjamin.abecassis@ens-lyon.fr

giving

$$\frac{I^{\text{on}}}{I^{\text{off}}} = 1 + \frac{3p_{\parallel} - \frac{6p_{\perp}}{1+D^r_{\parallel}/D^r_{\perp}}}{p_{\parallel} - p_{\perp} + q}. \tag{5}$$

## III. CALCULATION OF THE ROTATIONAL DIFFUSION CONSTANTS FOR ISOLATED AND STACKED NPL:

An isolated CdSe nanoplatelet (Fig. 1A) has the shape of a rectangular prism, with "bare" (i.e. without the ligand brush) dimensions $L_1^b = 20$ nm, $L_2^b = 9$ nm and $L_3^b = 1.5$ nm along the principal **1, 2** and **3-** axes, respectively. However, in the rotational diffusion process, the particle and the ligand brush reorient together as a single rigid body. So, the relevant dimensions are those of the "dressed" particle (i.e. including the ligand brush). Assuming that the ligands are evenly located all over the particle surface in a brush of 1.2 nm thickness, the dressed particle dimensions along the three axes, $L_i$, are respectively 22.4, 11.4, and 3.9 nm. To calculate the rotational diffusion coefficients of the dressed particle in hexane (with viscosity $\eta = 0.309 \times 10^{-3}$ Pa.s at room temperature), we approximate the particle as an equivalent ellipsoid with the same volume and axial ratios. Then, from the Perrin formulae [2, 3], we obtain $D_1^r = 1.8 \times 10^6$ s$^{-1}$, $D_2^r = 7 \times 10^5$ s$^{-1}$, $D_3^r = 7.6 \times 10^5$ s$^{-1}$ for the rotational diffusion constants $D_i^r$ around the axes i = **1, 2** and **3**. Therefore, the best uniaxial approximation for the reorientation of an isolated CdSe platelet is actually a rod with length $L_{\parallel} = L_1$, diameter $L_{\perp} = \sqrt{4L_2L_3/\pi}$ and approximate rotational diffusion constants $D^r_{\parallel} = 1.8 \times 10^6$ s$^{-1}$ and $D^r_{\perp} = 7.3 \times 10^5$ s$^{-1}$.

In a similar way, we calculated the three rotational diffusion constants for stacks of N platelets $D_i^r(N)$ versus the stack length $L_N = NL_3$. For values of $N > 20$, which are the experimentally relevant ones, even at short aging times (t = 25 days), the stacks behave as rod-like objects with long axis parallel to the 3-axis of the platelet. Then, $D^r_{\perp}$ is much smaller than $D^r_{\parallel}$ and its dependence on N is shown in Figure S1.

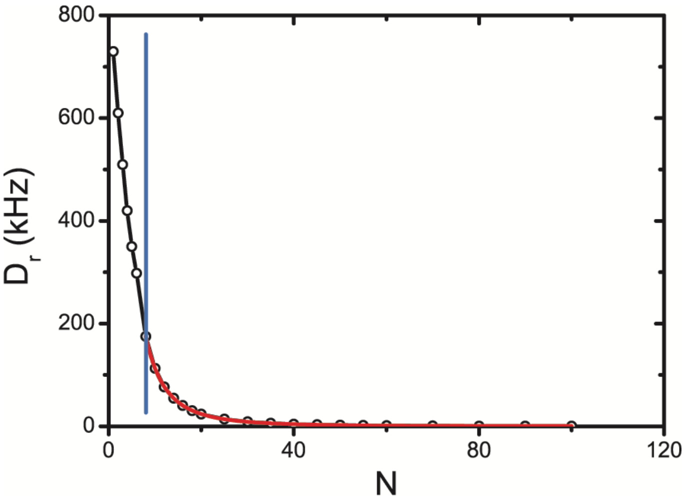


Figure 1: Calculated values, as a function of N, of the rotational diffusion constant of stacks of N CdSe platelets around an axis perpendicular to their revolution axis. The vertical blue straight line separates two domains where, at small N, the stacks have their revolution axis along the 1-axis and, at large N, the stacks have their revolution axis along the 3-axis. The black line is a guide to the eye whereas the red line is a fit of the data with a power-law dependence with an exponent close to -3 (-2.93).

## IV. ADDITIVITY OF THE COMPONENTS OF THE POLARIZABILITY TENSOR AT OPTICAL AND LOW FREQUENCIES

The additivity of the $\alpha_i$ components actually depends on the physical origin of the polarizability. Let us first consider the polarizability at optical frequencies, $\boldsymbol{\alpha^{opt}}$, which defines the refractive indices of the particle and its specific birefringence. The intrinsic birefringence of CdSe is small, $\Delta n^{\text{CdSe}} < 0.02$ [4], and can be neglected in front of the large form birefringence. The latter only depends on the particle shape, its average refractive index, $n^{\text{CdSe}} \simeq 2.69$,

and the refractive index of the solvent $n^s$=1.373 (strictly speaking the particle is surrounded by a thin ligand brush whose refractive index is close to that of the solvent). With the bare particle dimensions, the numerical calculation [5] gives $n_i^p = 2.51$, 2.35 and 1.85 for the specific particle indices along the principal axes i = 1, 2, 3 respectively. The rod-like approximation of an isolated particle leads to $\Delta n^p = n_\parallel^p - n_\perp^p = 0.39$. We underline that the biaxial optical polarizability tensor, $\boldsymbol{\alpha^{opt}}$, of the platelet is closer to an oblate tensor with revolution symmetry around the 3-axis, as expected for a disk, than to a prolate tensor with revolution symmetry around the 1-axis. The averaging process arising from the fast rotation of the platelet around its 1-axis makes the optical polarizability tensor prolate.

We now consider the polarizability of the particles and the stacks, $\boldsymbol{\alpha(f)}$, at low frequency (i.e. comparable to the field frequency), which is also important because it gives rise to the induced-dipole part of the field torque. Three different physical mechanisms mainly contribute to $\boldsymbol{\alpha(f)}$ in colloidal dispersions. The first one is due to the polarization of the bound charges at the particle surface because of the contrast of dielectric constant at the particle/solvent interface. This contribution, $\boldsymbol{\alpha}^{\mathbf{diel}}$ only depends on the aspect ratio of the particle and the dielectric contrast [6]. Similar to $\boldsymbol{\alpha^{opt}}$, $\boldsymbol{\alpha}^{\mathbf{diel}}$ for the stacks should be strictly additive because the dielectric constant of the ligand layer between the stacked particles is similar to that of the solvent. Moreover, $\boldsymbol{\alpha}^{\mathbf{diel}}$ should remain constant in the frequency range used here because its relaxation frequency is very high, close to the optical frequency range. The second mechanism, the Maxwell-Wagner (MW) polarization, is related to the accumulation on the particle surface of mobile (conductivity) charges when at least one of the two media has a finite conductivity [7, 8]. This contribution, $\boldsymbol{\alpha}^{\mathbf{MW}}$, can be very large when the conductivity contrast is high. If the particle is a perfect dielectric and the solvent has finite conductivity (as usually for aqueous dispersions), the relaxation frequency of this contribution, $f^{\mathrm{MW}}$, is of the order of magnitude of the charge relaxation frequency, $f^{\mathrm{ch}}$, of the solvent. Then, $\boldsymbol{\alpha}^{\mathbf{MW}}$ can be neglected in our external-electrodes experiment because the frequencies $f < f^{\mathrm{MW}}$ do not penetrate into the sample. In the present case, however, the semiconductor CdSe particles are dispersed in hexane, an almost perfect dielectric fluid, and the conductivity contrast is reversed. We then expect $f^{\mathrm{MW}} \gg f^{\mathrm{ch}}$, and the MW mechanism can give the main contribution to $\boldsymbol{\alpha^f}$ in this case. Moreover, we expect that the ligand brush has a low conductivity, similar to that of hexane, resulting in additivity of $\boldsymbol{\alpha}^{\mathbf{MW}}$ for the stacks. The third relaxation mechanism is that of Maxwell – Wagner - O'Konski (MWO) and is related to the polarization of the counter-ion atmosphere around a charged colloidal particle [9–11]. This contribution is particularly large for aqueous systems due to the large dissociating power of water and the resulting large surface charge of the particles. However, we expect this contribution to be negligible in our case, due to the apolar character of hexane.

## V. DISCUSSION OF THE RELATIONSHIP BETWEEN $N^{DC}$ AND $\mu_\parallel^N$

Despite the linear increase in time of both $N^{\mathrm{DC}}$ and $\mu_\parallel^N$, these quantities are not really proportional (see figure 6 of the main text), as would be expected from the relation $\mu_\parallel^N/N = \mu_3^1$. Indeed, this ratio is not constant but is significantly lower for the short stacks than for the long ones. This discrepancy can only be attributed partially to the stack polydispersity and is probably due to the presence, at short aging times, not only of small stacks but also of a large proportion of isolated particles. Let us consider a simple system consisting of isolated platelets with dipole moment $\sqrt{p_\parallel - p_\perp} \simeq \mu_\parallel^1$ and volume fraction $x\Phi$, and monodisperse stacks with the dipole moment $\mu_\parallel^N = N\mu_3^1$ and volume fraction $(1-x)\Phi$. The total induced birefringence is:

$$\Delta n = \Delta n^1 + \Delta n^N \simeq \frac{1}{15}\Phi \Delta n^p E^2 \left[ -x(\mu_\parallel^1)^2 + (1-x)(N\mu_3^1)^2 \right], \tag{6}$$

where we used the approximation $p_\parallel - p_\perp \gg \mid q \mid$ for both the stacks and the isolated particles. For the shortest stacks St1, we estimate from the size of the overshoot in Fig. 3A:

$$\Delta n^1/\Delta n^N \simeq -x_1(\mu_\parallel^1)^2/(1-x_1)(N\mu_3^1)^2 \simeq -0.1, \tag{7}$$

with $N \simeq 23$. For the longest stacks, St5, we assume that most platelets are stacked, $x \ll 1$, giving $\mu_3^1 \simeq \mu_\parallel^N/N \simeq 80D$ and from Eq (S7) we deduce that $x \simeq 0.8$ for the shortest stacks, meaning that most of the particles are still isolated. For the St2 stacks, there is still a small opposite-sign signal at the beginning of the on- and off- TEB curves, which indicates the presence of remaining isolated particles. The signal of the St3 stacks no longer shows this signature of isolated particles, so that $\mid \Delta n^1/\Delta n^N \mid < 0.01$. However, even in this case, with $N \simeq 32$ we only obtain $x < 0.45$. This shows that even such an important fraction of isolated particles is "invisible" in the TEB signal due to the much more efficient coupling of the stacked particles with the field.

We note that the $D_\perp^r$ value, as well as the $N^{\mathrm{DC}}$value deduced from it, are rather insensitive to the presence of isolated platelets because of the small amplitude of their induced birefringence, $\Delta n^1 \ll \Delta n^N$. Therefore, the presence of a

still large population of isolated particles in the early stacking stages explains the observed disagreement between the time evolutions of $\mu_{\|}^{N}$ and $N^{\mathrm{DC}}$.

---


[1] Ignacio Tinoco and Kiwamu Yamaoka. The Reversing Pulse Technique in Electric Birefringence. *The Journal of Physical Chemistry*, 63(3):423–427, 1959.

[2] Francis Perrin. Mouvement brownien d'un ellipsoide - I. Dispersion diélectrique pour des molécules ellipsoidales. *J. Phys. Radium*, 5(10):497–511, 1934.

[3] Francis Perrin. Mouvement Brownien d'un ellipsoide - II. Rotation libre et dépolarisation des fluorescences. Translation et diffusion de molécules ellipsoidales. *J. Phys. Radium*, 7(1):1–11, 1936.

[4] M. Schäffner, X. Bao, and A. Penzkofer. Principal optical constants measurement of uniaxial crystal CdSe in the wavelength region between 380 and 950 nm. *Applied Optics*, 31(22):4546–4552, August 1992.

[5] Masanori Abe and Manabu Gomi. Magneto-Optical Effect and Effective Dielectric Tensor in Composite Material Containing Magnetic Fine Particles or Thin Layers. *Japanese Journal of Applied Physics*, 23(12R):1580, December 1984.

[6] A. Peterlin and H. A. Stuart. *Zeitschrift fur Physik*, 112:129–147, March 1939.

[7] James Clerk Maxwell. *A Treatise on Electricity and Magnetism.* Cambridge University Press, Cambridge, reprint edition, 2010.

[8] Karl Willy Wagner. Erklärung der dielektrischen Nachwirkungsvorgänge auf Grund Maxwellscher Vorstellungen. *Archiv für Elektrotechnik*, 2(9):371–387, September 1914.

[9] Chester T. O'Konski. ELECTRIC PROPERTIES OF MACROMOLECULES. V. THEORY OF IONIC POLARIZATION IN POLYELECTROLYTES. *The Journal of Physical Chemistry*, 64(5):605–619, 1960.

[10] Chester T. O'Konski and Arthur J. Haltner. Characterization of the Monomer and Dimer of Tobacco Mosaic Virus by Transient Electric Birefringence [1]. *Journal of the American Chemical Society*, 78(15):3604–3610, 1956.

[11] Chester T. O'Konski and Sonja Krause. Theory of the Kerr constant of rigid conducting dipolar macromolecules. *The Journal of Physical Chemistry*, 74(17):3243–3250, 1970.
